# Supplementary material for: Cross-Input Certified Training for Universal Perturbations
Source: arXiv:2405.09176 source file (2024-09-09)
Supplement: Supplementary file 1 [file appendix.tex]

\documentclass[runningheads]{llncs}

\usepackage{silence}
%Disable all warnings issued by latex starting with "You have..."
\WarningFilter{latex}{You have requested package}

% ---------------------------------------------------------------
% Include basic ECCV package
 
% TODO REVIEW: Insert your submission number below by replacing '*****'
% TODO FINAL: Comment out the following line for the camera-ready version
%\usepackage[review,year=2024,ID=8210]{includes/eccv}
% TODO FINAL: Un-comment the following line for the camera-ready version
\usepackage{includes/eccv}

% OPTIONAL: Un-comment the following line for a version which is easier to read
% on small portrait-orientation screens (e.g., mobile phones, or beside other windows)
%\usepackage[mobile]{eccv}

% ---------------------------------------------------------------
% Other packages

% Commonly used abbreviations (\eg, \ie, \etc, \cf, \etal, etc.)
\usepackage{includes/eccvabbrv}

% Include other packages here, before hyperref.
\usepackage{graphicx}
\usepackage{booktabs}

% The "axessiblity" package can be found at: https://ctan.org/pkg/axessibility?lang=en
\usepackage[accsupp]{axessibility}  % Improves PDF readability for those with disabilities.

% ---------------------------------------------------------------
% Hyperref package

% It is strongly recommended to use hyperref, especially for the review version.
% Please disable hyperref *only* if you encounter grave issues.
% hyperref with option pagebackref eases the reviewers' job, but should be disabled for the final version.
%
% If you comment hyperref and then uncomment it, you should delete
% main.aux before re-running LaTeX.
% (Or just hit 'q' on the first LaTeX run, let it finish, and you
%  should be clear).

\usepackage{xr-hyper}
\makeatletter

\newcommand*{\addFileDependency}[1]{% argument=file name and extension
\typeout{(#1)}% latexmk will find this if $recorder=0
% however, in that case, it will ignore #1 if it is a .aux or 
% .pdf file etc and it exists! If it doesn't exist, it will appear 
% in the list of dependents regardless)
%
% Write the following if you want it to appear in \listfiles 
% --- although not really necessary and latexmk doesn't use this
%
\@addtofilelist{#1}
%
% latexmk will find this message if #1 doesn't exist (yet)
\IfFileExists{#1}{}{\typeout{No file #1.}}
}\makeatother

%------------End of helper code--------------

% put all the external documents here!
%\myexternaldocument{paper.tex}

% TODO FINAL: Comment out the following line for the camera-ready version
%\usepackage[pagebackref,breaklinks,colorlinks,citecolor=eccvblue]{hyperref}
% TODO FINAL: Un-comment the following line for the camera-ready version
\usepackage{hyperref}

% Support for ORCID icon
\usepackage{orcidlink}

\AddToHook{cmd/appendix/before}{%
  \setcounter{equation}{0}%
  \setcounter{theorem}{0}%
}
\usepackage{mathtools}
\usepackage{dashbox}
\usepackage{mathtools, amssymb, amsmath}
\usepackage{algorithm}
\usepackage[noend]{algorithmic}
\usepackage{booktabs}
\usepackage{multirow}
\usepackage{wrapfig}
\usepackage{tikz}

\usetikzlibrary{arrows.meta}
\definecolor{myblue}{HTML}{8aa9c6}

\definecolor{mygreen}{HTML}{B4E5A2}
\definecolor{myred}{HTML}{EEA3A3}
\definecolor{mydarkred}{HTML}{C00000}

\begin{document}

\appendix
\input{contents/appendix/proofs}
\input{contents/appendix/eval_details}

\end{document}
